# Supplementary material for: Numeracy for Language Models: Evaluating and Improving their Ability to Predict Numbers
Source: arXiv:1805.08154 source file (2018-05-21)
Supplement: Supplementary file 1 [file a-appendix.tex]

\subsection{Evaluation metrics}

Scale-dependent:

\begin{equation}
\label{eq:error}
e_{i} = v_i-\hat{v_i}
\end{equation}
\begin{equation}
\label{eq:rmse}
RMSE = \sqrt{\frac{1}{N}\sum_{i=1}^{N}e_i^2}
\end{equation}
\begin{equation}
\label{eq:mae}
MAE = \frac{1}{N}\sum_{i=1}^{N}|e_i|
\end{equation}
\begin{equation}
\label{eq:mdae}
MdAE = \median \{ |e_i| \}
\end{equation}

Scale-independent:
\begin{equation}
pe_{i} = \frac{v_i-\hat{v_i}}{v_i}
\end{equation}
\begin{equation}
\label{eq:mape}
MAPE = \frac{1}{N}\sum_{i=1}^{N}{
\left| pe_i \right|
}
\end{equation}
\begin{equation}
\label{eq:mdape}
MdAPE = \median \{ |pe_i| \}
\end{equation}
